# Supplementary material for: SimROD: A Simple Adaptation Method for Robust Object Detection
Source: arXiv:2107.13389 source file (2021-07-28)
Supplement: Supplementary file 1 [file pseudo_code_TG.tex]

\subsection{Diagram and pseudocode of the full framework}
In Section \ref{methods}, we provided a flow diagram in Fig. \ref{sys-diagram} and a pseudo-code in Algorithm \ref{algo:proposed}. Then, Sec. \ref{teacher-guided} introduced the teacher-guided pseudo-label mechanism (TG) in simple words. However, it was omitted from Fig. \ref{sys-diagram} and Algorithm \ref{algo:proposed} for ease of exposition. Here we provide the flow diagram and pseudo-code of the full framework including the TG in Fig. \ref{sys-diagram-TG} and Algorithm \ref{algo:proposed_TG}.\\

\begin{figure*}
\centering\includegraphics[width=0.7\paperwidth]{figures/SystemDiagram-teacher.jpg}\vspace{-4pt}
\caption{\small Flow diagram of the proposed full framework including the teacher-guided pseudo-label refinement}
\label{sys-diagram-TG}
\end{figure*}

\begin{algorithm}
\caption{\label{algo:proposed_TG}Proposed framework with teacher-guided pseudolabel refinement}
\begin{algorithmic}[1]
\algnewcommand\algorithmicinput{\textbf{Inputs:}}
\algnewcommand\INPUT{\item[\algorithmicinput]}
\algnewcommand\algorithmicoutput{\textbf{Output:}}
\algnewcommand\OUTPUT{\item[\algorithmicoutput]} 
\INPUT Source model {$\theta^{s}_{\tt M} $}, teacher model {$\theta^{s}_{\tt T} $}, labeled source data {$\cal D$}, unlabeled target data {$\cal \overline{D}$}, warmup epochs {$w$}, total epochs T, steps per epoch {$N$}, and batch size {$B$}
%\INPUT 
\OUTPUT Adapted model {$\theta^{a}_{\tt M} $}
\Procedure{Adapt}{$\theta^{s}_{\tt M},{\cal D},{\cal \overline{D}}$}

\State Adapt the teacher {$\theta^{s}_{\tt T} $} according to Algorithm \ref{algo:proposed}

\For{$\overline{\mathbf{x}}_{j}\gets \cal \overline{D}$}
	{$\overline{\mathbf{y}}_{j}\gets \text{GenPseudo}(\overline{\mathbf{x}}_{j}, \theta^{s}_{\tt T})$}
\EndFor

\State Initialize $\theta\gets {\theta^{s}_{\tt M}}$

\For{$layer\gets \theta.\text{layers}$}
	\If{layer is not BatchNorm}
		Freeze layer
	\EndIf
\EndFor

\For{$epoch\gets 1,\ldots, T$}
	\If{epoch == w}  \Comment{switch to Phase 2}
% 		\For{$\overline{x}\gets \cal \overline{D}$}
% 			{$\overline{\mathbf{y}}_{j}\gets \text{GenPseudo}(\overline{\mathbf{x}}_{j}, \theta^{s}_{\tt T})$}
% 		\EndFor
		\State Unfreeze all layers
	\EndIf
	
	\For{$\text{step}\gets 1,\ldots, N$}
		\State Sample a batch $\beta=\{(\mathbf{x}_{i},\mathbf{y}_{i})\}_{i=1}^{B}$  from $\cal D$
		\State {$\widehat{\beta} \gets \text{DomainMix}(\beta,{\cal \overline{D}}, \{\overline{\mathbf{y}}_{j}\})$} as in Algo 2.
		\State Update {$\theta $} to minimize the loss with $\widehat{\beta}$
	\EndFor
\EndFor
\State ${\theta^{a}_{\tt M}\gets \theta}$
\EndProcedure

\end{algorithmic}
\end{algorithm}

% \vfill

% \clearpage
