# Supplementary material for: SimROD: A Simple Adaptation Method for Robust Object Detection
Source: arXiv:2107.13389 source file (2021-07-28)
Supplement: Supplementary file 2 [file sourcecode.tex]

% \begin{minipage}{\linewidth}
\begin{figure*}[!b]
\centering\includegraphics[width=2.0\columnwidth]{supplementary/figures/demo.png}
\vspace{-4pt}
\caption{\small A screenshot of the provided demo application.}
\label{supp:demo_screenshot}
\end{figure*}
% \end{minipage}

\section{Code and demo}
\vspace{-4pt}

\subsection{Source code}
\vspace{-4pt}

We share our implementation code and some model checkpoints to make it easy to reproduce our work. The source-code is attached to the supplementary materials in a `code' dir. We also provide detailed instructions in a `README.md' file on how to train source models, adapt the source models to a target domain, run inference, and evaluate a model.

% \vspace{40pt}

\subsection{Demo}
\vspace{-4pt}

In addition to the code, we also include a `Demo.mp4' video file that contains a demonstration of our framework. This is based on screen recording of a web application we built to showcase few applications of our method to real-world scenarios. Our source-code contains the demo application and we plan to share the adapted model checkpoints later for running it in real-time with the given checkpoints.
