# Supplementary material for: SimROD: A Simple Adaptation Method for Robust Object Detection
Source: arXiv:2107.13389 source file (2021-07-28)
Supplement: Supplementary file 3 [file table_of_contents.tex]

\vspace{12pt}
\textbf{\large{Table of contents}} \vspace{4pt}\\
\textbf{6. Code and demo .......................................................... 11}\\
\indent \textbf{6.1. Source code ........................................................ 11}\\
\indent \textbf{6.2. Demo .................................................................. 11}\\
\textbf{7. Experiments setup .................................................... 11}\\
\indent \textbf{7.1. Training details and hyperparameters ........... 11}\\
\indent \textbf{7.2. More details on datasets ................................... 12}\\
\textbf{8. More results on synthetic-to-real and cross-camera \indent benchmarks .............................................................. 13}\\
\indent \textbf{8.1. Full results on Sim10K/KITTI to Cityscapes . 13}\\
\indent \textbf{8.2. Qualitative visualization ................................... 13}\\
\textbf{9. More results on artistic benchmark ........................ 13}\\
\indent \textbf{9.1. Benchmark results on Clipart and Comic ...... 13}\\
\indent \textbf{9.2. Data efficiency analysis on Watercolor and \indent \indent Comic .................................................................... 13}\\
\indent \textbf{9.3. Qualitative comparison on Clipart, Comic, and \indent \indent Watercolor ........................................................... 14}\\
\textbf{10. More results on image corruptions ....................... 16}\\
\indent \textbf{10.1. Results for different model sizes .................... 16}\\
\indent \textbf{10.2. Per-corruption performance on Pascal-C ..... 16}\\
\indent \textbf{10.3. Performance comparison with Augmix ......... 16}\\
\indent \textbf{10.4. Data efficiency analysis on Pascal-C .............. 17}\\
\indent \textbf{10.5. Effects of corruption severity levels ............... 21}\\
\indent \textbf{10.6. Qualitative comparison on image corruptions \indent \indent  ................................................................................ 21}\\
\indent \textbf{10.7. More detailed ablations on the components . 21}\\
\textbf{11. Dataset and DomainMix visualizations ................ 21}\\
